# Supplementary material for: The template-specific fidelity of DNA replication with high-order neighbor effects: a first-passage approach
Source: arXiv:1901.01495 source file (2019-04-08)
Supplement: Supplementary file 1 [file supplementarymaterial.pdf]

**The Supplementary Material of "The template-specific fidelity of DNA replication with high-order neighbor effects: a first-passage approach"**

The DNA template sequences and kinetic parameters used in the simulations and numerical computations are shown below. For the Markov chain template, the probability of consecutive $A$s (or $B$) is taken as 0.8 (a strong correlation).

| 1-10 | 11-20 | 21-30 | 31-40 | 41-50 |
|---|---|---|---|---|
| BAABAAABBB | AAAAABABAA | BBBBAAABBB | ABBABBAAAB | BBABAABAAA |
| 51-60 | 61-70 | 71-80 | 81-90 | 91-100 |
| BBBBBBABAA | ABBBBABABB | AAAABAABBB | ABBBBBBBBA | AABABABABB |

Random template

| 1-10 | 11-20 | 21-30 | 31-40 | 41-50 |
|---|---|---|---|---|
| AAAAAAAAAA | AAAAAAAAAA | BBBBBBBBBB | BBBBBBBBBB | BBBBBBBBBA |
| 51-60 | 61-70 | 71-80 | 81-90 | 91-100 |
| AAAAABBAAA | AAAAAAAAAA | AAABBBBBBB | BBBBBBBBBB | BBBAAAAAAA |

Markov template

TABLE I: kinetic parameters($s^{-1}$, simulation time unit)

| Parameters | 1 | | | | 2 | | | | 3 | | | |
|---|---|---|---|---|---|---|---|---|---|---|---|---|
| Template Pair | AA | AB | BA | BB | AA | AB | BA | BB | AA | AB | BA | BB |
| $k_{aa}$ | 65.0 | 45.0 | 76.0 | 45.0 | 250.0 | 0.42 | 0.52 | 0.0001 | 12344.0 | 55325.0 | 43.0 | 5436.0 |
| $k_{ab}$ | 68.0 | 45.0 | 64.0 | 97.0 | 0.77 | 200.0 | 0.0001 | 0.8 | 34.0 | 6325.0 | 2456.0 | 54.0 |
| $k_{ba}$ | 54.0 | 95.0 | 56.0 | 78.0 | 0.14 | 0.0001 | 150.0 | 0.56 | 3432.0 | 342.0 | 243.0 | 5456.0 |
| $k_{bb}$ | 45.0 | 66.0 | 80.0 | 67.0 | 0.0001 | 0.92 | 0.69 | 300.0 | 657890.0 | 3424.0 | 54.0 | 1324.0 |
| $r_{aa}$ | 12.0 | 23.0 | 7.0 | 4.0 | 0.0065 | 0.018 | 0.026 | 2.0 | 314.0 | 3244.0 | 543.0 | 32.0 |
| $r_{ab}$ | 16.0 | 24.0 | 16.0 | 4.0 | 0.033 | 0.0007 | 3.0 | 0.011 | 2.0 | 3.0 | 434.0 | 2.0 |
| $r_{ba}$ | 22.0 | 9.0 | 17.0 | 28.0 | 0.036 | 5.0 | 0.0018 | 0.067 | 3.0 | 4.0 | 543.0 | 234.0 |
| $r_{bb}$ | 14.0 | 23.0 | 12.0 | 19.0 | 2.0 | 0.046 | 0.098 | 0.0015 | 43.0 | 5.0 | 73.0 | 12.0 |

Parameters 1: the addition rates and deletions rates are of the same order of magnitude, which is different from the bio-conditions.

Parameters 2: bio-conditions in which $R$ and $W$ (base pairs) can be uniquely defined for each template unit (say $A$-$a$, $B$-$b$).

Parameters 3: all the rates are randomly assigned, which strongly violates the bio-conditions: no $R$ or $W$ can be properly defined for each template unit.

Fig.1-Fig.6 show more data on the comparison between the numerical results given by FP and IFS algorithm.

Fig.7 and Fig.8 show more data on the comparison between the precise and approximate numerical results of the positional probability and velocity given by FP algorithm.

Fig.9-Fig.11 show more data on the comparison between the precise and approximated fidelity profile given by FP algorithm.

Fig.12 shows the correlations and the relative correlations either for the random template or for the Markov template under different conditions.

In all these figures, the expanded template (i.e, the original template is repeated three times) is used in the FP algorithm, and only the middle copy is taken for the comparisons to eliminate the possible effects of the imaginary boundary conditions.

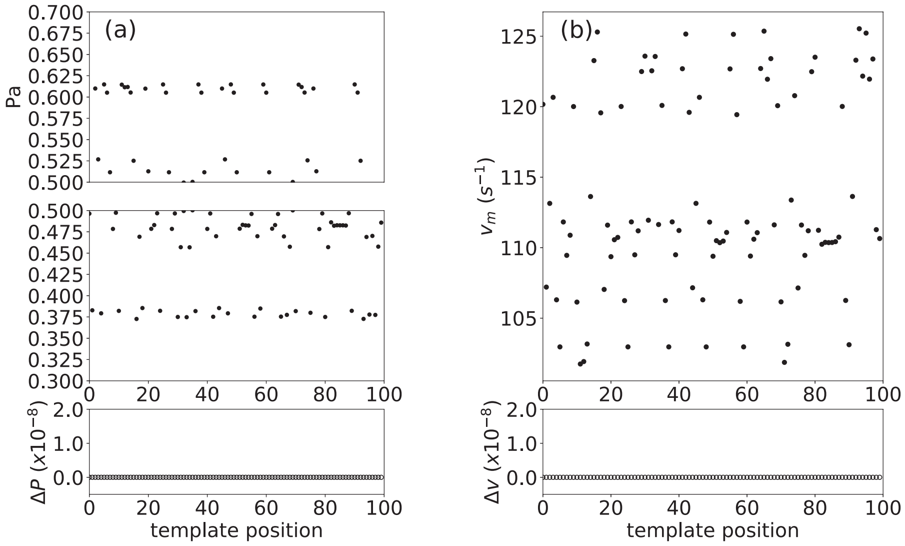


FIG. 1: Comparison between the numerical results given by FP and IFS algorithm, with the Parameters 1 and the random template. (a) (top)Pa for each position given by FP algorithm; (bottom) the relative difference $\Delta P = \max_{\alpha_m=a,b} |P_{\alpha_m}^{FP} - P_{\alpha_m}^{IFS}|/P_{\alpha_m}^{FP}$. (b) (top) $v_m$ for each position given by FP algorithm; (bottom) the relative difference $\Delta v_m = |v_{\alpha_m}^{FP} - v_{\alpha_m}^{IFS}|/v_{\alpha_m}^{FP}$

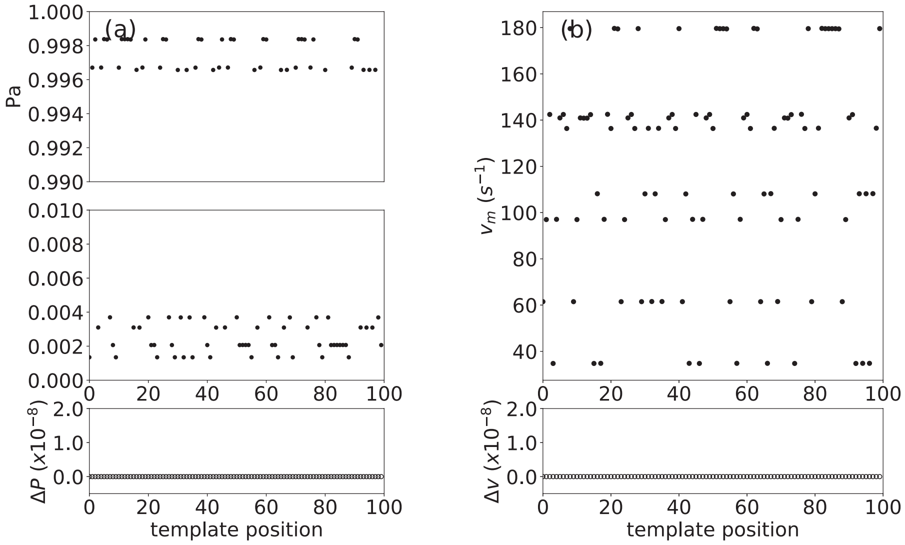


FIG. 2: Comparison between the numerical results given by FP and IFS algorithm, with Parameters 2 and the random template.

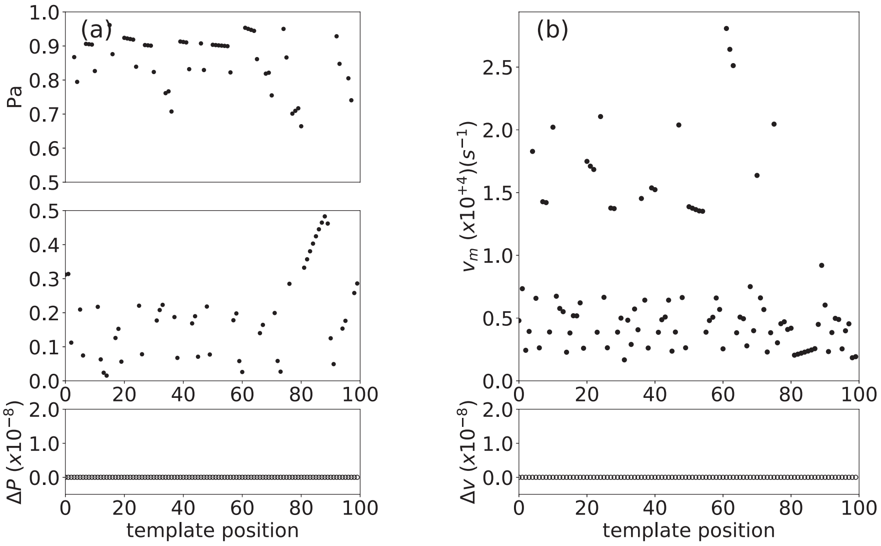


FIG. 3: Comparison between the numerical results given by FP and IFS algorithm, with the Parameters 3 and the random template.

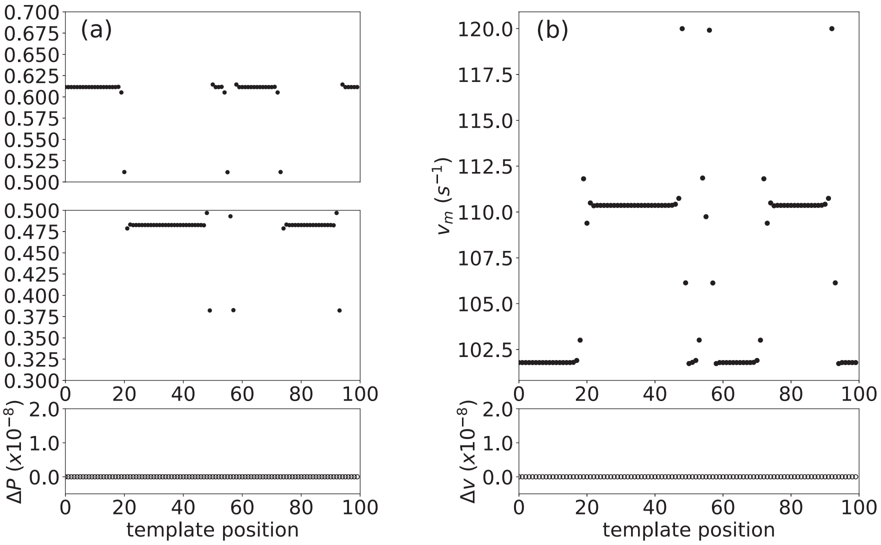


FIG. 4: Comparison between the numerical results given by FP and IFS algorithm, with Parameters 1 and the Markov template.

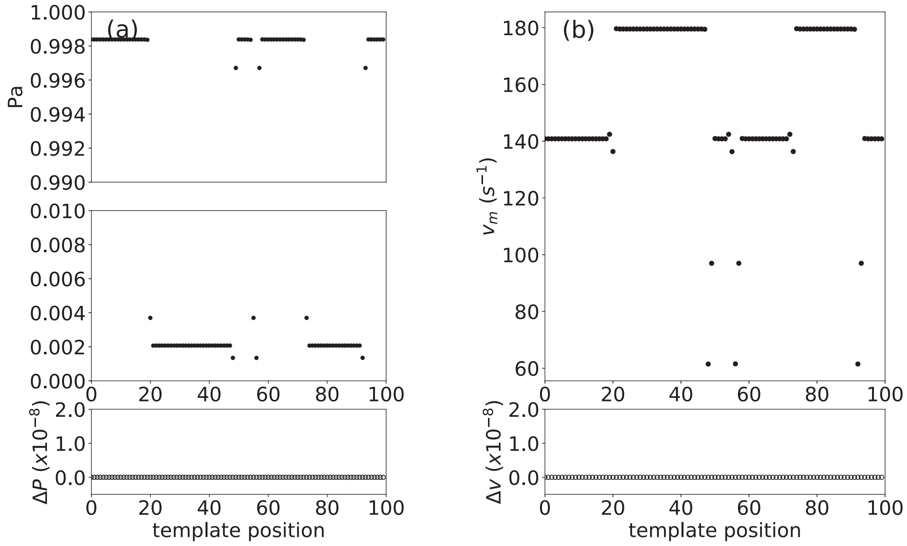


FIG. 5: Comparison between the numerical results given by FP and IFS algorithm, with Parameters 2 and the Markov template.

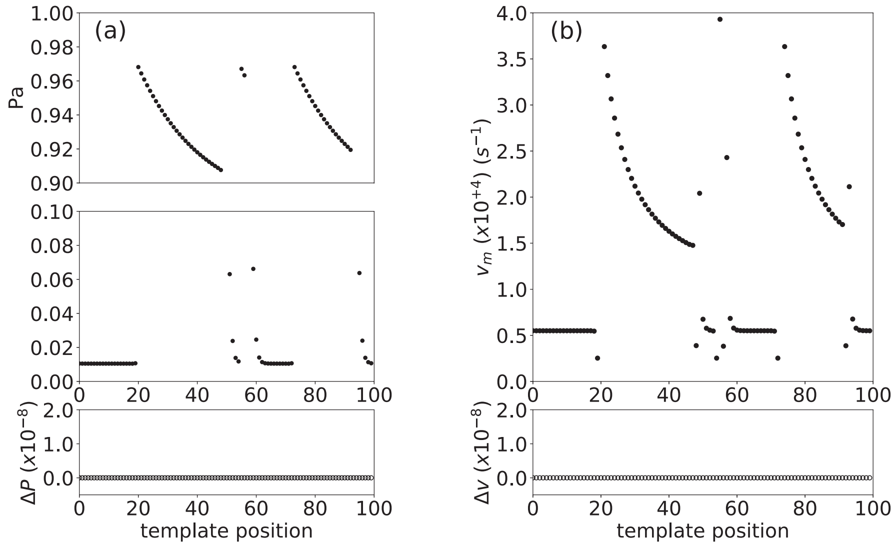


FIG. 6: Comparison between the numerical results given by FP and IFS algorithm, with Parameters 3 and the Markov template.

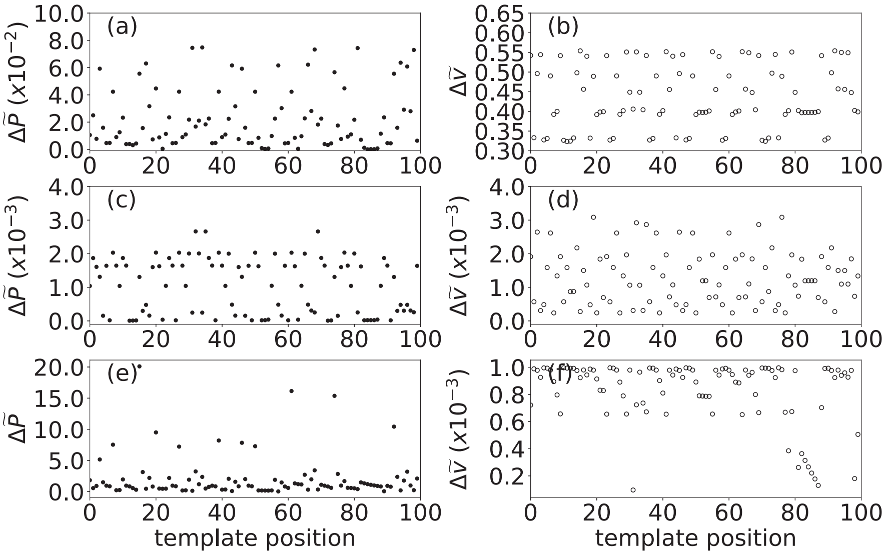


FIG. 7: Comparison between the precise (pre) and approximate (app) numerical results, for the random template. $\Delta\widetilde{P}_i = \max_{\alpha_i=a,b}\left(|P^{app}_{\alpha_i} - P^{pre}_{\alpha_i}|/P^{pre}_{\alpha_i}\right)$ and $\Delta\widetilde{v} = |v^{app} - v^{pre}|/v^{pre}$. (a)(b) $\Delta\widetilde{P}$, $\Delta\widetilde{v}$, under Parameter 1. (c)(d) $\Delta\widetilde{P}$, $\Delta\widetilde{v}$, under Parameter 2. (e)(f) $\Delta\widetilde{P}$, $\Delta\widetilde{v}$, under Parameter 3.

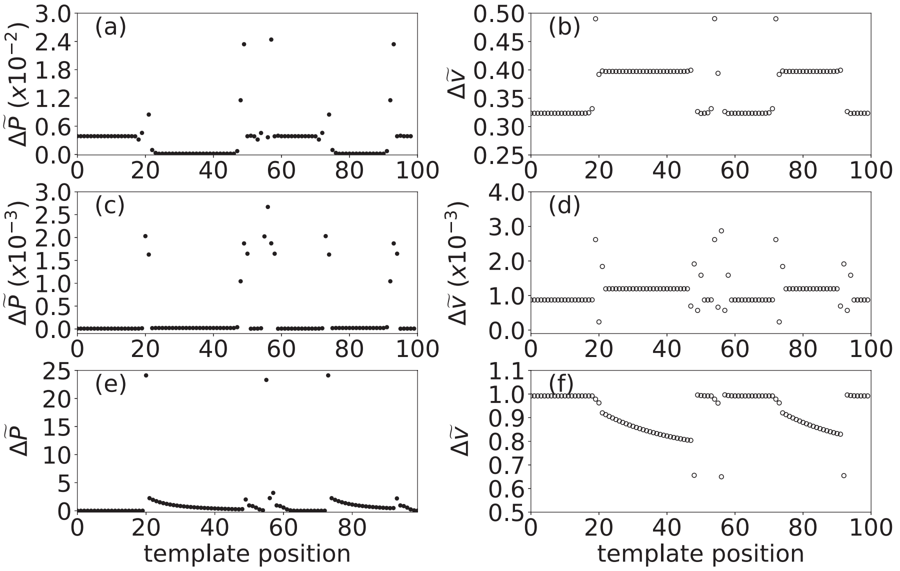


FIG. 8: Comparison between the precise (pre) and approximate (app) numerical results, for the Markov template. (a)(b) $\Delta\widetilde{P}$, $\Delta\widetilde{v}$, under Parameter 1. (c)(d) $\Delta\widetilde{P}$, $\Delta\widetilde{v}$, under Parameter 2. (e)(f) $\Delta\widetilde{P}$, $\Delta\widetilde{v}$, under Parameter 3.

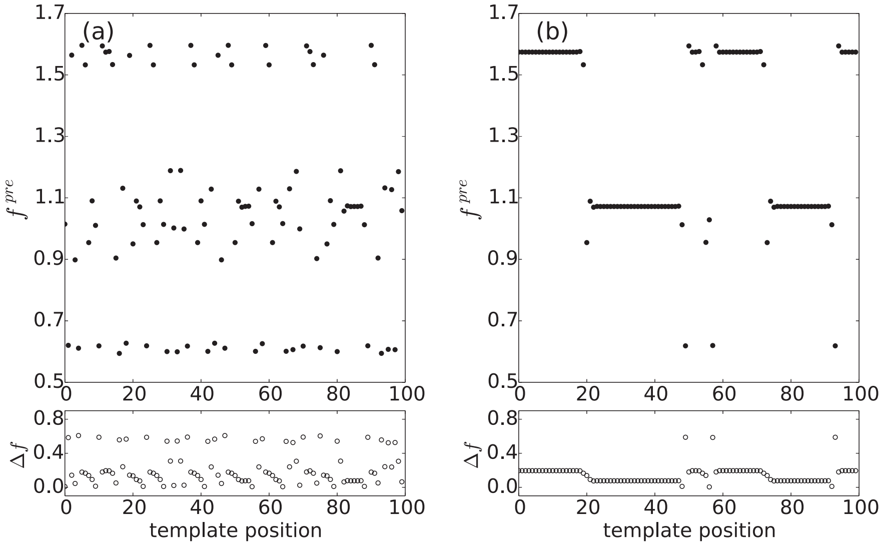


FIG. 9: Comparison between the precise(pre) and approximate(app) fidelity profile under Parameter 1 for the random template (a) and the Markov template (b). $\Delta f = |f^{pre} - f^{app}|/f^{pre}$.

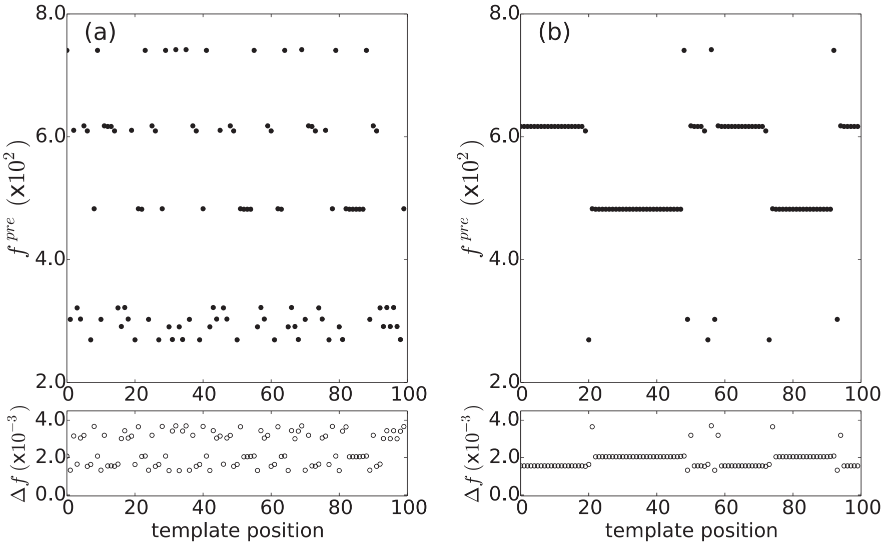


FIG. 10: Comparison between the precise(pre) and approximate(app) fidelity profile under Parameter 2 for the random template (a) and the Markov template (b).

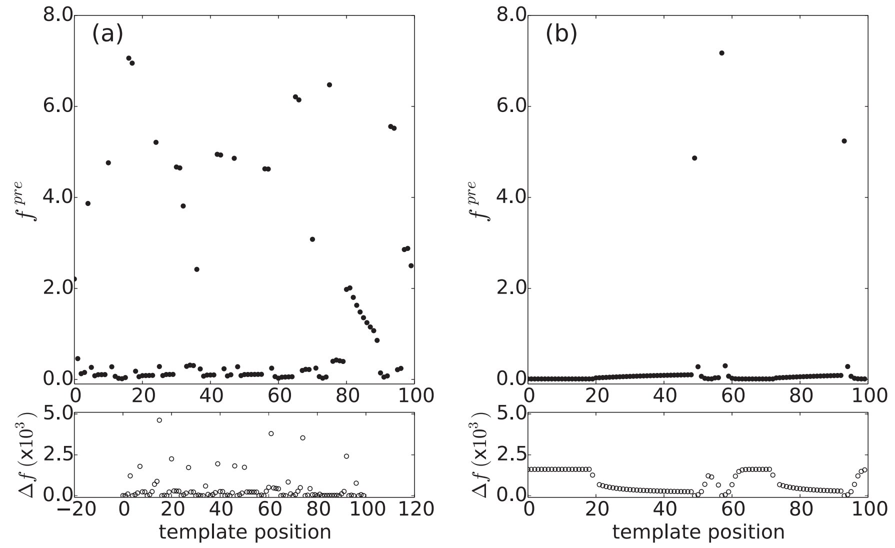


FIG. 11: Comparison between the precise(pre) and approximate(app) fidelity profile under Parameter 3 for the random template (a) and the Markov template (b).

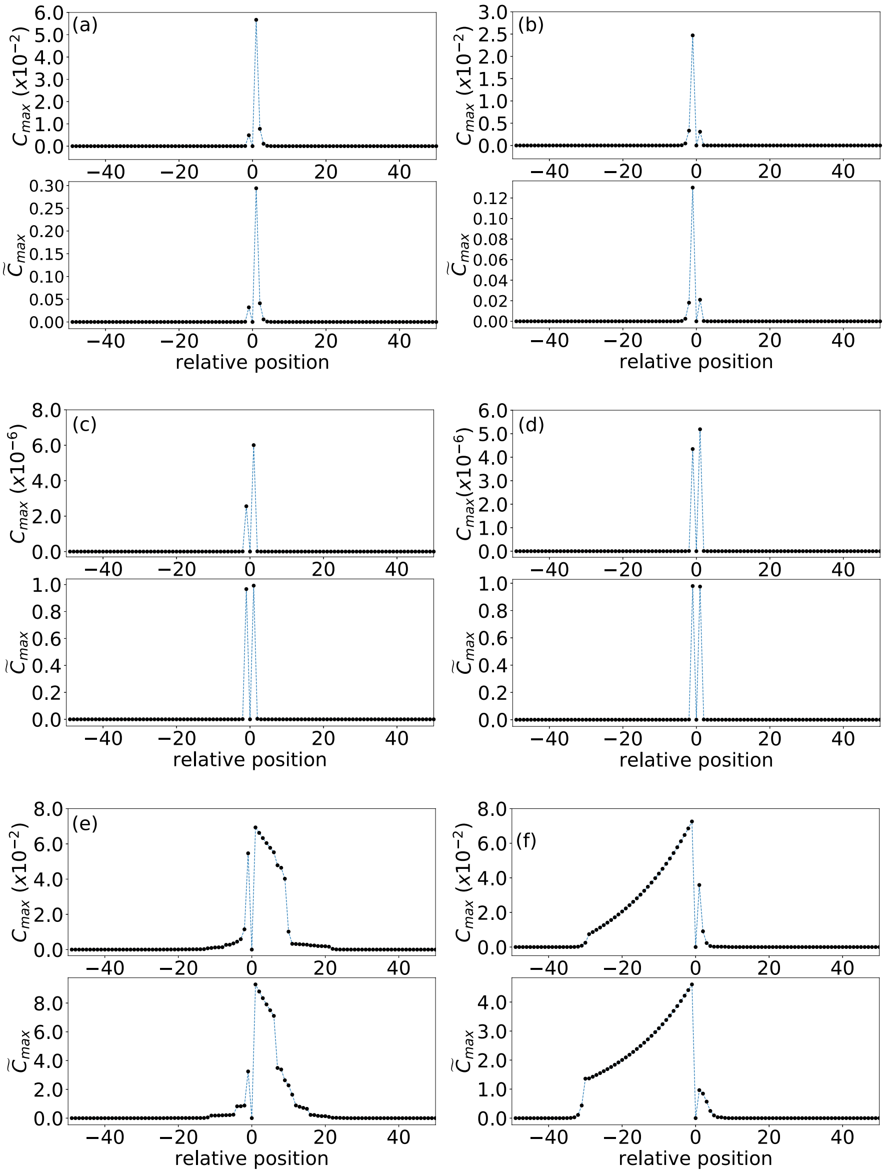


FIG. 12: The correlation $C_{max}$ and the relative correlation $\widetilde{C}_{max}$ between the position 50 and the rest positions of the template. (a)(c)(e) numerical results under Parameter 1,2,3, for the random template. (b)(d)(f) results under Parameter 1,2,3, for the Markov template.
